# Supplementary material for: Explicit formulas for forced convection in a shrouded longitudinal-fin heat sink with clearance
Source: arXiv:2412.09288 ancillary file (2024-12-12)
Supplement: Supplementary file 1 [file supplementary.pdf]

# Supplementary information for: Explicit formulas for forced convection in a shrouded longitudinal-fin heat sink with clearance

Toby L. Kirk<sup>†</sup>, Marc Hodes<sup>§</sup>

<sup>†</sup>*School of Mathematical Sciences, University of Southampton  
Southampton, SO14 3ZH, UK*

<sup>§</sup>*Department of Mechanical Engineering, Tufts University  
Medford MA, 02155, US*

## 1 Numerical method: 2D pseudospectral approach

In these materials we give further details of the numerical methods used to solve the full convection problem presented in the paper. As mentioned in the paper, the approach here is similar to that used and described by [1, 2] in slightly different contexts. Here we give an overview and emphasise the details that differ from the basic methodology within those references.

### 1.1 Nondimensional model equations

For convenience, we restate the velocity and temperature problems that are solved. The problem for the velocity field  $w(x, y)$  is given by

$$\frac{\partial^2 w}{\partial x^2} + \frac{\partial^2 w}{\partial y^2} = -1 \quad \text{in } \mathcal{D}, \quad (1)$$

$$w = 0, \quad \text{on } y = 0, 1 + c, \quad (2)$$

$$w = 0, \quad \text{on } x = 0, \varepsilon, \quad 0 < y < 1, \quad (3)$$

$$\frac{\partial w}{\partial x} = 0, \quad \text{on } x = 0, \varepsilon, \quad 1 < y < 1 + c. \quad (4)$$

Then the problem for the (scaled) temperature field  $\phi(x, y)$  (in the fluid) is

$$\left(\frac{w}{\bar{w}}\right) \lambda \phi = \frac{\partial^2 \phi}{\partial x^2} + \frac{\partial^2 \phi}{\partial y^2} \quad \text{in } \mathcal{D}, \quad (5)$$

$$\phi = 0, \quad \text{on } y = 0, \quad (6)$$

$$\frac{\partial \phi}{\partial y} = 0, \quad \text{on } y = 1 + c, \quad (7)$$

$$\frac{\partial \phi}{\partial x} = 0, \quad \text{on } x = 0, \quad 1 < y < 1 + c \quad (8)$$

$$\frac{\partial \phi}{\partial x} = 0, \quad \text{on } x = \varepsilon/2, \quad 0 < y < 1 + c. \quad (9)$$

which is coupled to the thermal problem for  $\phi_f(y)$  in the fin,

$$\Omega \frac{d^2 \phi_f}{dy^2} = - \left. \frac{\partial \phi}{\partial x} \right|_{x=0}, \quad \text{for } 0 < y < 1, \quad (10)$$

$$\phi_f = \phi|_{x=0}, \quad \text{for } 0 < y < 1, \quad (11)$$

$$\phi_f = 0, \quad \text{at } y = 0, \quad (12)$$

$$\frac{d\phi_f}{dy} = 0, \quad \text{at } y = 1, \quad (13)$$

with the eigenvalue  $\lambda$  to be determined,

$$\lambda = \frac{\varepsilon(1+c)}{\int_{\mathcal{D}} \left(\frac{w}{\bar{w}}\right) \phi dA}. \quad (14)$$

## 1.2 Domain decomposition and transformation

The domain is decomposed into 3 distinct subdomains (only 2 are relevant to the velocity problem) that are connect via conditions on their boundaries. These are the 2 rectangles comprising  $\{0 \leq y \leq 1, 0 \leq x \leq \varepsilon/2\}$  (domain 1) and  $\{1 \leq y \leq 1+c, 0 \leq x \leq \varepsilon/2\}$  (domain 2), but also the 1D line domain  $\{0 \leq y \leq 1, x = 0\}$  (domain 3) representing the fin. See Fig. 1. We only consider one half of one period,  $0 \leq x \leq 1/2$ , to reduce computational effort. Then the two rectangular subdomains (1 and 2) are mapped to  $[-1, 1] \times [-1, 1]$ , and the 1D subdomain (3) mapped to  $[-1, 1]$ , in order to use a Chebyshev collocation approach in each. The general transformation from a rectangular domain  $[x_-^{(n)}, x_+^{(n)}] \times [y_-^{(n)}, y_+^{(n)}]$  is

$$\xi^{(n)} = 2 \frac{x - x_-^{(n)}}{x_+^{(n)} - x_-^{(n)}} - 1, \quad \eta^{(n)} = 2 \frac{y - y_-^{(n)}}{y_+^{(n)} - y_-^{(n)}} - 1. \quad (15)$$

In particular, in subdomains  $n = 1, 2$  the new coordinates  $(\xi^{(n)}, \eta^{(n)}) \in [-1, 1] \times [-1, 1]$  are

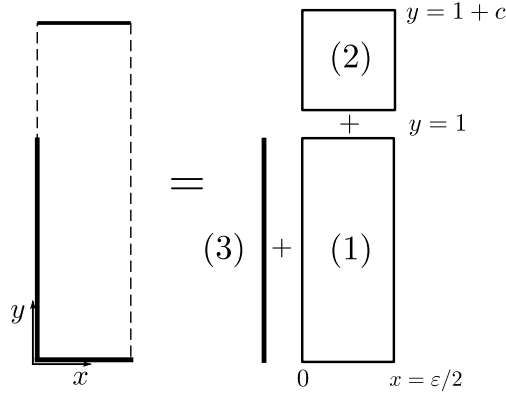

Figure 1: Diagram showing the domain decomposition of one half period into 3 subdomains: 2 rectangles (domains (1), (2)) and 1 line segment (domain (3)).

$$(\xi^{(1)}, \eta^{(1)}) = \left( \frac{4}{\varepsilon}x - 1, 2y - 1 \right), \quad (16)$$

$$(\xi^{(2)}, \eta^{(2)}) = \left( \frac{4}{\varepsilon}x - 1, \frac{2}{c}(y - 1) - 1 \right), \quad (17)$$

and that for the 1D subdomain is  $\eta^{(3)} = 2y - 1$ . Then, the equations and boundary conditions (1)-(4), (5)-(13) are transformed and applied in the appropriate subdomains, with all derivatives in each subdomain transforming via the chainrule. In general,

$$\frac{\partial}{\partial x} = \frac{2}{x_+^{(n)} - x_-^{(n)}} \frac{\partial}{\partial \xi^{(n)}}, \quad \frac{\partial}{\partial y} = \frac{2}{y_+^{(n)} - y_-^{(n)}} \frac{\partial}{\partial \eta^{(n)}}, \quad (18)$$

and in particular for each domain,

$$\text{Domain 1:} \quad \frac{\partial}{\partial x} = \frac{4}{\varepsilon} \frac{\partial}{\partial \xi^{(1)}}, \quad \frac{\partial}{\partial y} = 2 \frac{\partial}{\partial \eta^{(1)}}, \quad (19)$$

$$\text{Domain 2:} \quad \frac{\partial}{\partial x} = \frac{4}{\varepsilon} \frac{\partial}{\partial \xi^{(2)}}, \quad \frac{\partial}{\partial y} = \frac{2}{c} \frac{\partial}{\partial \eta^{(2)}}, \quad (20)$$

$$\text{Domain 3:} \quad \frac{\partial}{\partial y} = 2 \frac{\partial}{\partial \eta^{(3)}}. \quad (21)$$

Henceforth it is understood that the derivatives are transformed as above, but we will use the original notation (e.g.  $\partial/\partial x$ ) for brevity. In addition to transforming the original problem statement, we need additional continuity conditions on the common boundary between subdomains  $n = 1, 2$ , so we impose continuity of  $w^{(n)}$ ,  $\phi^{(n)}$  and their normal derivatives, e.g.

$$w^{(1)}|_{y=1} = w^{(2)}|_{y=1}, \quad \frac{\partial w^{(1)}}{\partial y} \Big|_{y=1} = \frac{\partial w^{(2)}}{\partial y} \Big|_{y=1}, \quad (22)$$

and similarly for  $\phi^{(n)}$ .

### 1.3 Discretization

We discretize each subdomain using a Chebyshev grid in each direction. In the 2D subdomains ( $n = 1$  and  $2$ ), we use a  $(N + 1) \times (M + 1)$  grid of points with the Gauss–Lobatto spacing,

$$(\xi_i^{(n)}, \eta_j^{(n)}) = (\cos(i\pi/N), \cos(j\pi/M)), \quad (23)$$

where  $i = 0, 1, \dots, N$  and  $j = 0, 1, \dots, M$ . Similarly for the 1D subdomain coordinate  $\eta_j^{(3)}$ . The transformed equations are imposed at the interior points ( $1 \leq i \leq N-1$ ,  $1 \leq j \leq M-1$ ) and the boundary conditions imposed when  $i = 0, N$  or  $j = 0, M$ . Consequently, the derivatives  $\partial/\partial\xi^{(n)}$  and  $\partial/\partial\eta^{(n)}$  are approximated by Chebyshev differentiation matrices  $\mathbf{D}_N(\xi^{(n)})$  and  $\mathbf{D}_M(\eta^{(n)})$  (see standard references e.g. [3, 4]) that act on solution vectors  $\mathbf{w}^{(n)} = (w_{00}^{(n)}, w_{01}^{(n)}, \dots)$  and  $\boldsymbol{\phi}^{(n)} = (\phi_{00}^{(n)}, \phi_{01}^{(n)}, \dots)$  representing the velocity and temperature values  $w_{ij}^{(n)}$  and  $\phi_{ij}^{(n)}$  at the grid points. These vectors are of length  $(N + 1)(M + 1)$ , except in subdomain 3 where only  $\boldsymbol{\phi}^{(3)}$  exists, and is of length  $M + 1$ .

#### 1.3.1 Velocity problem

The velocity problem is linear and consists of 2 subdomains. The discretized Poisson equation in subdomain  $n = 1, 2$  can be written  $\mathbf{L}^{(n)}\mathbf{w}^{(n)} = \mathbf{f}^{(n)}$  where the  $(N + 1)(M + 1) \times (N + 1)(M + 1)$  square matrix  $\mathbf{L}^{(n)}$  encodes the (transformed) Laplacian operator and the vector  $\mathbf{f}^{(n)}$  encodes the uniform forcing of  $-1$  at each point. However, the rows of each corresponding to the boundary points are replaced with the boundary conditions there. The corner points can be included with either boundary of the subdomain, but here we group the corners with the lower or upper faces. As all boundary conditions are homogeneous, the rows of  $\mathbf{f}^{(n)}$  are replaced with zeros. Notably, the continuity of  $w$  condition is enforced at the top of domain (1), and continuity of the derivative at the bottom of domain (2). Then the system for the velocity is

$$\begin{pmatrix} \mathbf{L}^{(1)} & \mathbf{L}^{(1,2)} \\ \mathbf{L}^{(2,1)} & \mathbf{L}^{(2)} \end{pmatrix} \begin{pmatrix} \mathbf{w}^{(1)} \\ \mathbf{w}^{(2)} \end{pmatrix} = \begin{pmatrix} \mathbf{f}^{(1)} \\ \mathbf{f}^{(2)} \end{pmatrix}, \quad (24)$$

where  $\mathbf{L}^{(1,2)}$  is a result of the continuity of  $w$  condition between (1) and (2), and  $\mathbf{L}^{(2,1)}$  a result of the continuity of the derivative. The above system is then inverted using backslash in MATLAB to find the values of the velocity field. Integration to find the flow rate (and hence average velocity) is done in each subdomain using Clenshaw–Curtis weights for quadrature, and then summed.

#### 1.3.2 Thermal problem

The temperature problem is nonlinear and has 3 subdomains (compared to 2 for the velocity), and thus is slightly more complicated. It is also nonlinear, so we solve it in an iterative manner. Given a proposed thermal solution  $(\phi_k, \phi_{f,k}, \lambda_k)$  at a given iteration step  $k$ , then new solutions for the temperature fields  $(\phi_{k+1}, \phi_{f,k+1})$  at step  $k + 1$  are found by solving the

$\phi$  problem but where the advective part of (5), i.e.  $\lambda_k(w/\bar{w})\phi_k$  is assumed known from the previous order:

$$\left(\frac{w}{\bar{w}}\right)\lambda_k\phi_k = \frac{\partial^2\phi_{k+1}}{\partial x^2} + \frac{\partial^2\phi_{k+1}}{\partial y^2} \quad \text{in } \mathcal{D}. \quad (25)$$

Then  $\lambda_{k+1}$  is computed using  $\phi_{k+1}$  in (14). This allows us to treat the problem as linear in  $(\phi_{k+1}, \phi_{f,k+1})$  at every step.

The problems for  $(\phi_k, \phi_{f,k})$  at step  $k$  are discretized in a similar way to the velocity problem. In subdomains  $n = 1, 2$ , the governing equation for  $\phi_{k+1}^{(n)}$  can be written

$$\mathbf{Q}^{(n)}\phi_{k+1}^{(n)} = \mathbf{g}_k^{(n)}, \quad (26)$$

where the  $(N+1)(M+1) \times (N+1)(M+1)$  square matrix  $\mathbf{Q}^{(n)}$  encodes the Laplacian operator and  $\mathbf{g}_k^{(n)}$  the known advective forcing  $\lambda_k(w_{ij}^{(n)}/\bar{w})\phi_{k,ij}^{(n)}$  at the grid points  $i, j$ . Again, the rows of  $\mathbf{Q}^{(n)}$  and  $\mathbf{g}_k^{(n)}$  corresponding to boundary points are replaced with the boundary conditions. The connection (continuity) conditions between subdomains (1) and (2) are handled in the same way as for the velocity problem, giving connection matrices  $\mathbf{Q}^{(2,1)}$  and  $\mathbf{Q}^{(1,2)}$ . In the additional subdomain, for 1D conduction in the fin, the solution at step  $k+1$  is denoted  $\phi_{k+1}^{(3)}$  (a vector of length  $M+1$ ), and the fin equation (10) discretizes to

$$\mathbf{Q}^{(3)}\phi_{k+1}^{(3)} = -\mathbf{Q}^{(3,1)}\phi_{k+1}^{(1)}, \quad (27)$$

where  $\mathbf{Q}^{(3)}$  is  $(M+1) \times (M+1)$  and  $\mathbf{Q}^{(3,1)}$  is  $(M+1) \times (N+1)(M+1)$ . The first and last rows of each are replaced by the condition at the top ( $\partial\phi^{(3)}/\partial y = 0$ ) and bottom ( $\phi^{(3)} = 0$ ) of the fin. Lastly, temperature continuity between the fin (domain (3)) and fluid (domain (1)) is enforced as a condition in domain (1), which gives rise to the matrix  $\mathbf{Q}^{(1,3)}$ . The resulting system is

$$\begin{pmatrix} \mathbf{Q}^{(1)} & \mathbf{Q}^{(1,2)} & \mathbf{Q}^{(1,3)} \\ \mathbf{Q}^{(2,1)} & \mathbf{Q}^{(2)} & \mathbf{0} \\ \mathbf{Q}^{(3,1)} & \mathbf{0} & \mathbf{Q}^{(3)} \end{pmatrix} \begin{pmatrix} \phi^{(1)} \\ \phi^{(2)} \\ \phi^{(3)} \end{pmatrix}_{k+1} = \begin{pmatrix} \mathbf{g}^{(1)} \\ \mathbf{g}^{(2)} \\ \mathbf{0} \end{pmatrix}_k. \quad (28)$$

Note that  $\mathbf{Q}^{(1,3)}$  and  $\mathbf{Q}^{(3,1)}$  are (the only) non-square matrices on the left-hand side, as they connect subdomains with a different total number of grid points. This system is inverted to give  $\phi_{k+1}^{(n)}$ , then  $\lambda_{k+1}$  computed from (14). The procedure is repeated until  $\lambda_k$  changes by less than 0.01%, with typically less than 10 iterations required.

## References

- [1] S. E. Game, M. Hodes, T. L. Kirk, and D. T Papageorgiou. Nusselt numbers for poiseuille flow over isoflux parallel ridges for arbitrary meniscus curvature. *J. Heat Trans-T ASME*, 140:081701, 2018.

- [2] Michael D. Mayer, Jonah Kadoko, and Marc Hodes. Two-Dimensional Numerical Analysis of Gas Diffusion-Induced Cassie to Wenzel State Transition. *Journal of Heat Transfer*, 143(10):103001, 09 2021.
- [3] R. Peyret. *Spectral Methods for Incompressible Viscous Flow*, volume 148 of *Applied Mathematical Sciences*. Springer Science & Business Media, 2013.
- [4] L. N. Trefethen. *Spectral Methods in MATLAB*. SIAM, 2000.
